# Supplementary material for: Learning Density Distribution of Reachable States for Autonomous Systems
Source: arXiv:2109.06728 source file (2021-09-14)
Supplement: Supplementary file 1 [file baks.tex]

\subsection{Ground robot navigation}

\begin{figure}[!htbp]
\centering
\includegraphics[width=0.32\textwidth]{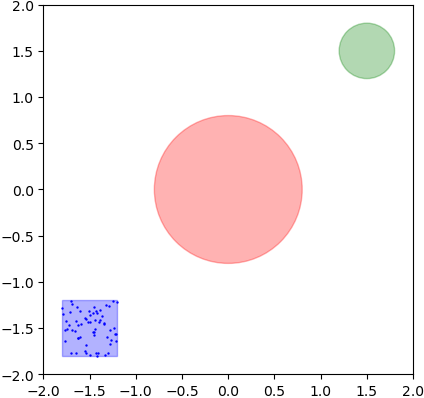} \hfill
\caption{Screenshot of the ground robot experiment. The robot starting from the initial condition (blue) needs to reach the goal (shown in green) while avoiding the obstacle (shown in red).}
\label{fig:screenshot}
\end{figure}

Here we consider an experiment for a ground robot navigation problem. The robot starting from a uniform distribution in $S_{init}$ (blue) needs to go to the goal state $S_{goal}$ (green), while avoiding the obstacle $S_{obstacle}$ (red), as shown in Fig.~\ref{fig:screenshot}. We assume the supply function is zero in this case. The robot state $(x,y,\theta, v)$ denotes the x ,y coordinates, heading angle and the velocity. The robot's dynamics follows a Dubins car model:
\begin{equation}
    \begin{cases}
    \dot{x}=v\cos(\theta)\\
    \dot{y}=v\cos(\theta)\\
    \dot{\theta} = u_{\theta}(x,y,\theta,v)\\
    \dot{v} = u_v(x,y,\theta, v)\\
    \end{cases}
\end{equation}

In this experiment, we set $S_{init}=\{-1.8\leq x\leq-1.2,\,-1.8\leq y\leq -1.2, 0.0\leq \theta \leq \pi/2, 0.0\leq v \leq 1.0\}$, $S_{goal}=\{(x-1.5)^2+(y-1.5)^2\leq 0.09\}$ and $S_{obstacle}=\{x^2+y^2\leq 0.64\}$.

We use our reachable set distribution framework introduced in Sec.~\ref{sec:rpm} to analyze for a pretrained NN controller for the robot task. We collect $N=1000$ trajectories with trajectory length $T=50$ in the simulator using this NN controller for the robot. We randomly choose 800 for training and 200 for validation. Our dynamics and density neural network is a fully-connected neural network with 2 hidden layers with 32 hidden units in each layer. We train our neural network on the training set for 30 minutes on an NVidia RTX 2080Ti GPU and observe no substantial decrease in validation error then. Next we use RPM to partition the input space into 4772 cells in 10 seconds (we also save the output cells and corresponding affine mapping matrices). Finally we leverage this partition result to compute for the system's reachable set distribution and to perform online verification.

\section{Appendix B}
\noindent{\textbf{System forward reachable set distribution:}} We use RPM to compute the forward and backward reachable sets for our trained neural network introduced in Sec.~\ref{sec:nn}. Recall that our neural network estimates the dynamics as well as the density gain, taking the initial state $x_0$ and time $t$ as input. Therefore, by computing the forward reachable set for an input polyhedron $S^i$
% \dawei{\marginnote{\DRAFT{(Solved)} How about explicitly pointing out that $i$ is not an index but short for ``input"?}}
(we denote the superscript ${(\cdot)}^i$ short for ``input", and the superscript ${(\cdot)}^o$ is short for ``output" ): 
\begin{equation}
\{(x_0,t)| A_x x_0\leq b_x,\,T_{\text{begin}}\leq t \leq T_{\text{end}}\}
\label{eq:fwd-cell}
\end{equation}
we are able to answer the question of ``where and at what density will the state reach during time span $[T_{\text{begin}},T_{\text{end}}]$, from the initial state region $\{x_0|A_x x_0\leq b_x\}$?". 

To solve the question above, we use RPM to compute a set of $M$ possible input polyhedral cells $\{S^i_k\}_{k=0}^{M-1}$ (where $\bigcup\limits_{k=1}^M S^i_k = S^i$) and the corresponding $M$ output polyhedral cells $\{S^o_k\}_{k=0}^{M-1}$, such that for each $k$, the NN is an affine transform from $S_k^i$ to $S_k^o$. Recall that the first dimension of our neural network output estimates the intermediate density gain (as shown in Eq.~\eqref{eq:transform}), and the rest dimensions estimate the future state, thus we can explicitly write out $S^o_k=\{(z, x)|A_k \begin{pmatrix} z \\ x  \end{pmatrix}\leq b_k\}$.
% \dawei{\marginnote{\DRAFT{(Solved)} $z=\text{NN}_{[0:1]}(x_0,t)$ looks a bit strange. $z$ is a free variable and should not be defined using this equation. How about ``where $z$ is the first element of the NN's output which denotes the intermediate ...". Also, how about spelling out the shape of $A_k$ and $b_k$?}}
This representation indicates that each output set $S_k^o$ unveils the density bound locally in its corresponding system forward reachable set in the state space: for each output polyhedron $S^o_k$, the system forward reachable set $S^{o,x}_k$ can be computed by projecting the output polyhedral cell to the state space:
\begin{equation}
S^{o,x}_k=\{x|(x,z)\in S^o_k \},
\label{eq:fwd-state}
\end{equation}
% \dawei{\reversemarginpar\marginnote{\DRAFT{(Solved)} Formally define Proj?
% or just define the ``$[]$" operator for a vector, i.e., $x[i:j]$ is a slice of $x$. Then, instead of $NN_{[i:j]}(\cdot)$, we use $NN(\cdot)[i:j]$.}}
and the upper-bound for the density can be solved via a linear program:
\begin{equation}
\begin{cases}
    z_{k,max} = \text{max} z \\
    \text{s.t.} A_k \begin{pmatrix} z \\ x  \end{pmatrix}\leq b_k
\end{cases}
\label{eq:fwd-dens-1}
\end{equation}
and the lower-bound $z_{k,min}$ can be derived in a similar fashion, by just replacing the ``$\max$" operator to the ``$\min$" operator. Then the corresponding density bound $[\rho_{k,min}, \rho_{k,max}]$ for the system forward reachable set $S^{o,x}_k$ can be computed by:
\begin{equation}
\begin{cases}
    \rho_{k,min}=\min(e^{(z_{k,min} \cdot T_{\text{begin}})}, e^{(z_{k,min}\cdot T_{\text{end}})})\\
    \rho_{k,max}=\max(e^{(z_{k,max} \cdot T_{\text{begin}})}, e^{(z_{k,max}\cdot T_{\text{end}})})
    \end{cases}
    \label{eq:fwd-dens-2}
\end{equation}

Finally the system forward reachable set can be represented as a union of projected output polyhedral cells: $\mathop{\bigcup}\limits_{k=0}^{M-1} S^{o,x}_k$ where each cell $S^{o,x}_k$ is associated with a density bound $[\rho_{k, min},\rho_{k,max}]$. Notice that the density bound depends on both the query time span $[T_{\text{begin}}, T_{\text{end}}]$ and the feasible region $A_k\begin{pmatrix} z \\ x \end{pmatrix}\leq b_k)$. Therefore, to maintain a tighter density bound, one can further divide the input polyhedra cells $S^i_k$ or check on a narrower time span.

\noindent{\textbf{System backward reachability verification}} 
Using the backward reachability analysis from RPM, we can verify whether the initial condition of the system will lead to an unsafe terminal state (e.g. collision) under certain density range, which is useful for safety verification. 

Denote an unsafe terminal state by $S_{unsafe}=\{x \in \mathcal{X}|A_{q,x} x \leq b_{q,x}\}$ and a density constraint by $\rho_{min}\leq\rho\leq\rho_{max}$. We want to verify that for a given time span $T_{begin}\leq t\leq T_{end}$, the initial condition won't lead the system to $S_{unsafe}$ with density $\rho_{min}\leq\rho\leq\rho_{max}$.

We first derive the range of the neural network's intermediate density prediction $z$ (as shown in Eq.~\eqref{eq:transform}), which should be:
\begin{equation}
    \begin{cases}
       z_{min}=\min((\log \rho_{min})/T_{begin}, (\log \rho_{min})/T_{end})\\
       z_{max}=\max((\log \rho_{max})/T_{begin}, (\log \rho_{max})/T_{end})
    \end{cases}
\end{equation}
thus the unsafe output for our neural network should be:
\begin{equation}S_{unsafe, NN}=\{\begin{bmatrix}z \\ x\end{bmatrix} | A_{q,x}x\leq b_{q,x}, z_{min}\leq z \leq z_{max}\}
\end{equation}

To check whether the neural network will produce the unsafe output defined above, we need to check the intersection between the output polyhedron cells $\{S_k^o\}_{k=0}^{M-1}$ and the unsafe output polyhedron $S_{unsafe,NN}$. If there is no intersection, then we can verify that the system from the initial condition won't reach the unsafe terminal state for a given density range.

Directly checking for all polyhedral intersections is slow, because each intersection check between the two polyhedra $\{x|A_1x\leq b_1\}$ and $\{x|A_2x\leq b_2\}$ is equivalent to checking for the feasibility of a linear programming with constraints $A_1x\leq b_1, A_2 x\leq b_2$, which has the complexity of $O(n^3L)$ when using interior point methods with $n$ variables and $L$ length of a binary coding of the input data \citep{potra2000interior}. To accelerate the verification process, we use a hyper-rectangle-based heuristic to reduce the number of polyhedral intersection check. We first pre-process each output cell $S^o_k$ to a hyper-rectangle $R^o_k$, by obtaining each cell's vertices and compute the min/max values in each dimension. For each query $S_{unsafe,NN}$, we first compute its outer hyper-rectangle $R_{unsafe,NN}$, then we check the intersection of the hyper-rectangles between $R_k^o$ and $R_{unsafe,NN}$, where each pairwise-checking can be done in $O(n)$ with $n$ being the number of variables. If no intersection is found, then we can verify that the system is safe. Otherwise, only for the intersected hyper-rectangle pairs will we do the polyhedral intersection checking. From the experiment we show that this heuristic saves up to 70\% of the computation time.

\noindent{\textbf{System reachable set probability computation}}
%The RPM \cite{vincent2020reachable} computes the piecewise-affine representation of the neural network $y=NN(v)$ as $\{A_k,b_k,C_k, d_k, E_k, f_k\}_{k=1}^N$ where under each input polyhedron $H^k_0=\{v|A_k v\leq b_k\}$, the neural network can be seen as an affine mapping $y=C_k v+d_k$ hence the corresponding output set is also a polyhedron $H^k_t=\{y|E_k y\leq f_k\}$. Here $v=\begin{pmatrix} x \\ t \end{pmatrix}$ is the concatenation of the state vector $x$ and the scalar $t$ (representing the time). For an arbitrary system initial condition $S_{init}={x|Ax\leq b}$ with initial density $\rho_{init}$, its forward reachable set at time $\tau$ will be an union of the intersection between the polyhedron $P_{init}=\{(x,t)^T|x\in S_{init},t=\tau\}$ and all the 

% \dawei{\DRAFT{(Solved)} Add a paragraph here to define the problem we want to solve in this section.}

Given an initial state distribution, we want to figure out the probability distribution of the system forward reachable sets, as well as the probability for the states land into a queried set.

The RPM \cite{vincent2020reachable} computes the piecewise-affine representation of the neural network as $\{(A_k,b_k,C_k, d_k, E_k, f_k)\}_{k=1}^N$, where for each input cell: $H_k=\{v|A_k v \leq b_k\}$, the neural network can be seen as an affine mapping: $y=C_k v + d_k$, which results the output cell also a polyhedron: $M_k=\{y|E_k y\leq f_k\}$. 

For an arbitrary probability density function (whose support is bounded), we can approximate it using the input polyhedral cells\footnote{We can always further divide those input cells to make the bound tighter/ more precise, while still guaranteeing the Neural Network on each cell can be seen as an affine transformation.} defined above with bounded state densities $\{(H_k, \rho_{k}^{min}, \rho_k^{max})\}_{k=1}^{N}$, 
% \dawei{\marginnote{\DRAFT{(Solved: yes you are right.)} Is it necessary to introduce this partition $\{(S_j^{init}, \rho_{i}^{min}, \rho_j^{max})\}_{j=1}^{N_\rho}$? Why do not we use solely the partition computed by RPM and compute $\rho^{min}$, $\rho^{max}$, $g^{min}$ and $g^{max}$ in each cell? In this way, we can avoid introducing $C_k$ and so on.}}
where for each state in $H_k$, the state density is always between $\rho_{k}^{min}$ and $\rho_k^{max}$. For the state initialized from the polyhedra $H_k$, its forward reachable set at time $\tau$ will be: $M_{k}^{\tau}=\left\{y|y=C_k v + d_k, v=\begin{pmatrix}x \\ \tau\end{pmatrix}, x\in H_k\right\}$. For each $M_{k}^{\tau}$, we can derive the system state space $S_{k}$ and the range of the corresponding density gain $[g^{min}_{k}, g^{max}_{k}]$ using Eq.~\eqref{eq:fwd-state} and Eq.~\eqref{eq:fwd-dens-1}. Finally, the joint probability for the state initialized from $H_k$ and reaches $S_{k}$ is bounded by $\left[P_{k}^{min},P_{k}^{max}\right]$:
\begin{equation}
    \begin{cases}
       P_{k}^{min}= \text{Vol}(S_{k}) \rho_k^{min} g^{min}_k \\
       P_{k}^{max}= \text{Vol}(S_{k}) \rho_k^{max} g^{max}_k 
    \end{cases}
\end{equation}
where $\text{Vol}(\cdot)$ computes the volume for a polyhedron. By computing for all input cells $\{H_k\}_{k=1}^N$, we can derive the system forward reachable set and the corresponding probability bound as $\left\{(S_{k}, P_{k}^{min}, P_{k}^{max})\right\}_{k=1:N}$.

The backward reachable set probability can be computed in a similar fashion, by checking the intersection between the query output region and the output cells derived by RPM, compute each intersection's probability range by its volume and the density bound, and finally aggregate the probability of all those intersections.

%For each input polyhedron $S^k_0$, to compute the reachable set $S^k_t$ at time $t$, we can first compute the polyhedron intersected with the time constraint: $\tilde{S}^k_0=S^k_0\cap \{\}$
